# Supplementary material for: DM-VIO: Delayed Marginalization Visual-Inertial Odometry
Source: arXiv:2201.04114 source file (2022-01-11)
Supplement: Supplementary file 1 [file supplementary.pdf]

# Additional evaluations for DM-VIO: Delayed Marginalization Visual-Inertial Odometry

Lukas von Stumberg and Daniel Cremers

We provide an ablation study on different parts of the IMU initializer in section I, an ablation study on the impact of the dynamic photometric weight in section II, and runtime results in section III.

## I. ABLATION IMU INITIALIZER

We perform an ablation study on various parts of the IMU initializer. In particular, we compare to the following three baselines, which build on top of each other, meaning that everything removed in baseline  $n$  is also removed in baseline  $n + 1$ .

- 1) We remove the Reinitialization and the Marginalization replacement, corresponding to the orange and the yellow boxes in Fig. 3 of the main paper. Note that the scale is still optimized in the main system after initialization.
- 2) No readvancing: We do not replace the marginalization prior of the main graph after the first initialization. This means that in the purple box "Initialize" in Fig. 3 of the main paper we only replace the values and not the marginalization prior of the main graph. Instead we add a constant prior on the initial scale, which is necessary for the scale to not immediately diverge afterwards.
- 3) No PGBA: We remove the "PGBA IMU Init" and directly initialize with the result of the Coarse IMU Init.

The experiments are performed in non-realtime mode in order to not be dependent on the particular machine.

The results on the 4Seasons dataset are shown in Fig. S1. With each ablation the result becomes significantly worse, showing that all parts of the method contribute to the results. In particular we observe that the proposed delayed marginalization is very important, as it is the foundation of both the pose graph bundle adjustment (PGBA) and the readvancing (and subsequently also the marginalization replacement).

For completeness we should mention that on TUM-VI and EuRoC the contributions do not bring a significant performance improvement, as both datasets are much less challenging for the IMU initialization.

## II. ABLATION DYNAMIC PHOTOMETRIC WEIGHT

We provide ablation studies showing the effect of the dynamic photometric weight proposed in the main paper. For this we disable the dynamic part and always use the constant weight  $W = \lambda$  (of course  $\lambda$  is set to the same value as for the other results). In Fig. S2a we compare to the results shown in the main paper on TUM-VI, both runs are in realtime mode.

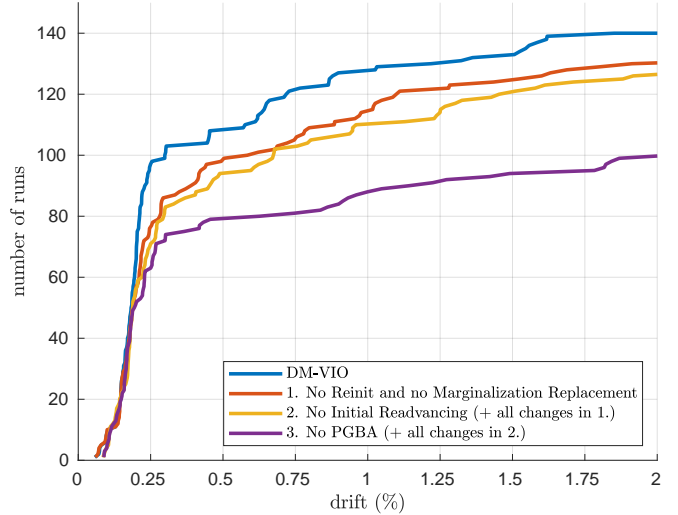

Fig. S1: Ablation study on various parts of the IMU initializer on the 4Seasons dataset (non-realtime). Removing the reinitialization and the marginalization replacement (1.) makes a significant difference, as the marginalization prior can become inconsistent if the initial scale estimate is off. Removing also the initial marginalization replacement powered by readvancing (2.) further deteriorates the performance. Removing the pose graph bundle adjustment and only using the Coarse IMU init (3.) makes the biggest difference. This ablation shows the significance of delayed marginalization which is the foundation of PGBA, readvancing and marginalization replacement.

It can be seen that the dynamic weights improve the overall robustness of the method. The effect is most visible on the TUM-VI slides (Fig. S2b, S2c), where the version without dynamic weights does not work well in 4 of the 15 runs whereas our method works well in all runs. The dynamic weighting is designed for situations where the image quality gets really bad. On the other datasets, significant degradation of image quality is rare, hence there is only a marginal difference for them.

## III. RUNTIME

We perform extensive runtime analysis on the same MacBook Pro 2013 (i7 at 2.3GHz) that was used for generating the results in the main paper. For each part of the method we save the mean time and standard deviation it takes while processing a sequence. We run our method in real-time mode 10 times on each sequence of EuRoC dataset, resulting in 110 recorded means and standard deviations for each part.

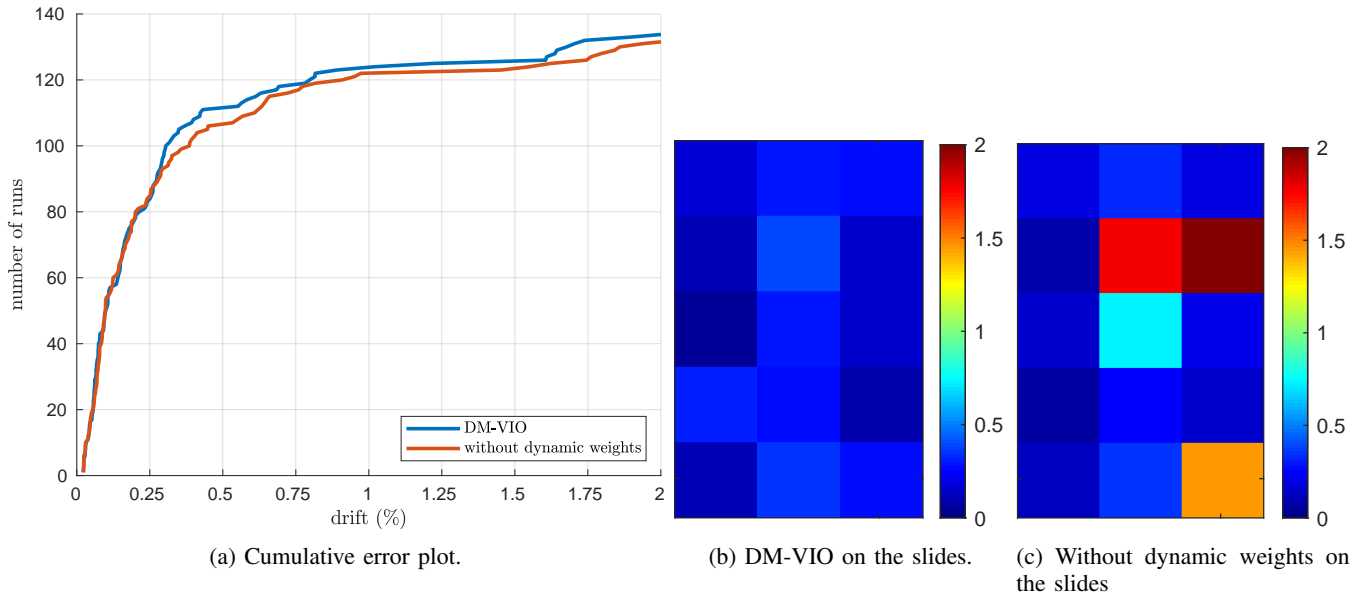

Fig. S2: Realtime results on the TUM-VI dataset with and without the dynamic photometric weights. a) Cumulative error plot. The dynamic weight provides a noticeable improvement in robustness. Only few sequences contain hard enough images to trigger the dynamic weight, hence the overall improvement can appear small. However for these hard sequences, success rate is increased. b) and c): Each colored square represents the drift (%) for one of the 5 runs (rows) on the three slides sequences (columns). With dynamic weights our method works well for all 30 runs whereas the version without them fails once and accumulates a large drift for three executions.

TABLE S1: We save runtime statistics for different parts of the method and show the mean over all 110 runs on the EuRoC dataset (10 times on each sequence). Top 2 sections: Runtime for the two main threads. Bottom 3 sections: Runtime for the parts of the IMU initializer, which are performed occasionally. Note that the overhead introduced by our initializer is small: The only regular overhead is the delayed marginalization, taking 0.44ms which amounts to 0.8% of the keyframe operations. Both, the Coarse IMU initializer and the PGBA initializer perform most operations in a separate thread when running. The only relevant overhead in the keyframe thread is after a successful PGBA and during a marginalization replacement.

| Component                                            | Part                                       | Mean time (ms)<br>Mean of 110 runs | Standard deviation (ms)<br>Mean of 110 runs |
|------------------------------------------------------|--------------------------------------------|------------------------------------|---------------------------------------------|
| Coarse Tracking<br>Performed for every frame.        | Total                                      | 10.34                              | 10.16                                       |
|                                                      | Direct Image Alignment                     | 4.70                               | 1.31                                        |
|                                                      | Build Image Pyramid                        | 4.78                               | 0.52                                        |
| Keyframe Operations<br>Performed for every keyframe. | Total                                      | 53.67                              | 6.89                                        |
|                                                      | Bundle Adjustment                          | 26.49                              | 5.57                                        |
|                                                      | Create Candidate Points                    | 5.83                               | 0.38                                        |
|                                                      | Trace candidate points                     | 4.37                               | 1.83                                        |
|                                                      | Activate new points                        | 3.56                               | 0.77                                        |
|                                                      | Keyframe Marginalization (full)            | 3.24                               | 0.5                                         |
|                                                      | — Drop residuals, recompute adjoints, etc. | — 1.71                             | — 0.39                                      |
|                                                      | — Marginalize main graph                   | — 0.61                             | — 0.10                                      |
|                                                      | — <b>Delayed marginalization</b>           | — 0.44                             | — 0.20                                      |
| Coarse IMU Init                                      | Runtime in separate thread                 | 9.08                               | 5.63                                        |
|                                                      | Overhead Coarse Tracking thread            | 0.05                               | 0.04                                        |
| PGBA (Re-)init                                       | Runtime in separate thread                 | 74.11                              | 24.77                                       |
|                                                      | — Optimization                             | — 54.72                            | — 23.40                                     |
|                                                      | — Readvancing                              | — 7.61                             | — 1.37                                      |
|                                                      | Overhead Keyframe thread when active       | 0.17                               | 0.04                                        |
|                                                      | Overhead Keyframe thread after success     | 14.50                              | 8.52                                        |
|                                                      | — Include KFs added while PGBA was running | — 13.15                            | — 8.52                                      |
|                                                      | — Readvancing of the newly added KFs       | — 1.35                             | — 0.19                                      |
| Marginalization Replacement                          | Total (Keyframe Thread)                    | 21.02                              | 8.98                                        |
|                                                      | Build Graph                                | 1.15                               | 0.45                                        |
|                                                      | Readvance                                  | 19.87                              | 8.97                                        |

We present the mean mean runtime and the mean standard deviation over the 110 runs in Table S1.

Even on the relatively old machine the overall runtimes are quite fast. The tracking could run at 97 FPS on average and the keyframe processing could run at 19 FPS. Note that the dataset is recorded at only 20 FPS, and to work well our method needs to process 5-6 keyframes per second.

The only regular overhead introduced by our initializer is the delayed marginalization, which amounts to 0.8% of the total processing time of each keyframe. The Coarse IMU initializer and the PGBA both run in separate threads when active. We do note that after a successful PGBA, some processing has to be done in the keyframe thread in order to include the keyframes, which have been bundle adjusted while the PGBA was running. Similarly the marginalization replacement currently runs in the keyframe thread. However both of these parts are comparably fast (14.50ms and 21.02ms respectively), and are performed only a few times during every run.
